# Supplementary material for: Climatic Phase Transitions Unravel the Onset and Withdrawal of Indian Monsoon
Source: arXiv:2503.15148 source file (2025-03-20)
Supplement: Supplementary file 1 [file supplementary_material.pdf]

# Supplementary Information of Climatic Phase Transitions Unravel the Onset and Withdrawal of Indian Monsoon

Yogenraj Patil<sup>1, 2</sup>, Gaurav Chopra<sup>1, 2</sup>, Shruti Tandon<sup>1, 2</sup>, B. N. Goswami<sup>3</sup>, and  
R. I. Sujith<sup>1, 2</sup>

<sup>1</sup>Department of Aerospace Engineering, Indian Institute of Technology  
Madras, Chennai-600036, India

<sup>2</sup>Centre of Excellence for studying Critical Transitions in Complex Systems,  
Indian Institute of Technology Madras, Chennai-60036, India

<sup>3</sup>Department of Physics, Gauhati University, Guwahati-781014, India

# 1 Various definitions of onset and withdrawal of the Indian Monsoon

The Monsoon season, by convention, is defined as the seasonal accumulation of rainfall in addition to the seasonal reversal of winds. The onset and withdrawal of monsoon demarcate the beginning and end of the rainy season, respectively. Local-scale and regional-to-large-scale are the two main scales that have been adopted in the past to calculate the length of the rainy season<sup>1</sup>. The local-scale methods involve using local information, such as the precipitation at a given location. In addition to precipitation, the regional or large-scale methods are based on an additional thermodynamic parameter, such as the temperature averaged over a large region. However, the problem with defining the onsets in these individual scales is that the local-scale methods lack connectivity with the large-scale ITCZ structure and often lead to false onsets whereas the large-scale methods cannot be used to track the progression of monsoon since they are based on averaging over a large area. Some of the local and regional-to-large-scale definitions used in the literature to define the onset and withdrawal of the Indian monsoon are mentioned below:

1. Misra *et al.*<sup>2</sup> (2018): The minima and maxima of the daily cumulative precipitation anomaly at a location for a given year indicate the local onset and the local withdrawal of the monsoon, respectively. Since this method incorporates precipitation at each individual location in a region, it is based on a local scale.
2. Xavier *et al.*<sup>3</sup> (2007): The shifting of deep tropospheric heat source from south to north denotes the onset and vice-versa for the withdrawal, respectively. This definition is based on the reversal in the gradient of tropospheric temperature (averaged between 600 hPa to 200 hPa) between Southern region (15°S-5°N, 40°E-100°E) and Northern region (5°N-35°N, 40°E-100°E). This approach was further extended to redefine the regional-scale onset of NEI by Saha *et al.* (2023)<sup>4</sup>, where the Northern region mentioned above was divided into two regions: Central India (40°E-89°E) and Northeast India (89°E-100°E). This definition is a regional scale definition since it is based on the average of tropospheric temperature over a large region.
3. IMD method: The India Meteorological Department (IMD) defines the onset of monsoon

over Kerala (MoK) based on the following three criteria<sup>5</sup>:

- I. **Rainfall:** The rainfall at 60% of the 14 locations: Minicoy, Amini, Allapuzha, Kollam, Kochi, Kozhikode, Kannur, Kudulu, Punallur, Thalassery, Thrissur, Thiruvananthapuram, and Mangalore should be equal to or greater than 2.5 mm for two consecutive days after 10<sup>th</sup> May. The onset over Kerala is then declared on the 2<sup>nd</sup> day, given the below two conditions (II and III) are also satisfied.
- II. **Wind field:** The westerly winds should be present from sea level to 600 hPa altitude in the geographical region from 0°N-10°N, 55°E-80°E. Furthermore, the zonal wind speed of these westerly winds at 925 hPa altitude in the region from 5°N-10°N, 70°E-80°E must be of the order of 15-20 knots.
- III. **Outgoing Longwave Radiation (OLR):** The OLR value in the geographical region from 5°N-10°N, 70°E-80°E should be below 200 Wm<sup>-2</sup>.

The withdrawal of southwest monsoon defined by the IMD is given based on the synoptic scale observations over the western parts of Northwest India:

- I. There should be no rainfall activity over a region for a consecutive period of 5 days.
- II. An anticyclonic circulation must be established from sea level to 850 hPa altitude.
- III. Significant drop in moisture content in satellite water vapour imageries and tephigrams (or the skewT-ln P) charts.

The definition of MoK used by the IMD to define the onset over the Indian peninsula is a regional scale definition. The above definition of IMD has evolved over the past decades<sup>5-8</sup>.

4. Fasullo and Webster<sup>9</sup> (2003): They define a Hydrological Onset and Withdrawal Index (HOWI), which is a regional scale definition based on vertically integrated moisture transport over the Arabian Sea and Southwest India. The day when HOWI changes from negative to positive values is defined as the onset and vice versa for withdrawal.
5. Walker and Bordoni<sup>10</sup> (2016): This study involves the use of horizontal moisture flux convergence (MFC) to determine the large-scale onset of monsoon over India. It uses a

two-phase linear regression model to detect the change points of the cumulative MFC (CMFC), which correspond to the large-scale onset and withdrawal. In addition to the above, the local onset and withdrawal are found by the same method but replacing the CMFC with cumulative precipitation averaged over a  $4^\circ \times 4^\circ$  geographical region centred around every grid point to smoothen the small-scale variability. They show that the local onsets in Kerala are progressively later than the large-scale onset, whereas, for the regions in Northeast India, local-scale onsets occur 1 month after the large-scale onset.

6. Wang and LinHo<sup>11</sup> (2002): This study utilizes the mean rainfall of the climatological pentad with global coverage of  $2.5^\circ \times 2.5^\circ$ . They define the relative mean rainfall rate of the pentad ( $RR_i$ ) by

$$RR_i = R_i - R_{JAN}, \quad i = 1, 2, 3, \dots, 73 \quad (1)$$

where  $R_{JAN}$  is the mean precipitation rate of January, and  $R_i$  is the mean precipitation rate of the pentad. The Julian pentad in which  $RR_i$  exceeds (and drops below) five  $\text{mmd}^{-1}$  is defined as the onset pentad (and withdrawal pentad).

## 2 Usefulness of Climate Networks

A complex system comprises multiple constituent subsystems that interact with each other and exhibit features such as self-organization, emergence, nonlinearity, and critical phenomena. Complex systems theory<sup>12–15</sup> is an interdisciplinary approach with a wide range of applications in climate<sup>16–21</sup>, engineering<sup>22</sup>, sociology<sup>23</sup>, and economics<sup>24</sup>. The dynamics and transitions in the patterns occurring in complex systems are effectively analysed and studied using complex networks. A complex network consists of nodes connected through links. Nodes represent the constituent subsystems, and links represent interactions between them. These links are established based on the extent of similarity and causality, which include measures such as correlation, mutual information, and event synchronization.

In the past two decades, networks have been extensively used in climate science to unravel teleconnections such as the ENSO<sup>25</sup> and analyse and predict various climate phenomena<sup>26</sup>. In a climate network, the geographical locations are considered nodes, and the links encode information about the connectivity across these nodes. The construction of a climate network involves considering the climate as a grid of oscillators<sup>27</sup>. Every oscillator in a climate network is considered a dynamical system that varies in a complex way. The characteristics of the first climate network constructed using 500 hPa pressure data were similar to that of the small world network<sup>27</sup>, with the overall dynamics emerging due to the interactions between two different subsystems: tropics and extratropics. The tropical network was fully connected, while the network in the extratropics exhibited scale-free characteristics and multifractal properties<sup>27</sup>. The network-based approaches in climate sciences have been recently used to improve the prediction of El Nino events<sup>28–31</sup>, extreme rainfall events in the Indian summer monsoon<sup>32,33</sup>, the eastern Central Andes<sup>34,35</sup>, droughts in the Central Amazon region<sup>36</sup>, heatwave patterns and propagations<sup>37</sup>, and the extreme stratospheric polar vortex states<sup>38</sup>.

Here, we emphasize the previous studies that involved precipitation networks. Malik *et al.*<sup>32,39</sup> identified interactions of different atmospheric processes responsible for the generation of extreme rainfall events over South Asia using event synchronization. They also distinguished the regions of coherent rainfall activity during the active and break phases of the Indian summer monsoon. Scarsoglio *et al.*<sup>40</sup> constructed a correlation-based precipitation network and analysed the spatial variation of rainfall across the globe. They found that small-scale extreme

events are rare over the Sahel and East Australian region due to low rainfall events and, therefore, emerge as supernodes with very high connectivity. On the other hand, the Southeast Asian region exhibits short-range connectivity due to the high frequency of extreme events such as tropical cyclones, monsoons, and heat waves. Stolbova *et al.*<sup>33</sup> utilized event synchronization measures and discovered three regions: North Pakistan, Tibetan Plateau, and Eastern Ghats, which are strongly responsible for the origin of extreme rainfall events over the Indian peninsula. Boers *et al.*<sup>34</sup> revealed the main moisture pathways and major convergence zones of the South American monsoon system using event synchronization. These include the South American Low-Level Jet, ITCZ, and the South Atlantic Convergence Zone. They also identified the mesoscale convective cluster storms along with the deep convection areas in the Amazon basin. Another study by Boers *et al.*<sup>41</sup> that involved the use of event synchronization measures unravels Rossby waves as the physical mechanism behind the extreme rainfall teleconnections between Europe and South Central Asia.

### 3 Phase Transitions in Complex Systems using Network Theory

A phase is a dynamically stable state of a system, and a phase transition occurs when a substance transforms from one state of matter to another. In nature, the phase transitions occur to minimize the free energy of a system. Conventionally, phase transitions are studied in the context of equilibrium systems. However, in the case of complex systems, phase transitions are usually studied in non-equilibrium systems<sup>42</sup>. Here, the phase represents the collective state of multiple interacting subsystems. One or more control parameters govern the state of the system as a whole. A control parameter is a variable that can be adjusted to control or modify the behaviour of a system. For example, the concentration of carbon dioxide gas ( $\text{CO}_2$ ) acts as a primary control parameter for climate change today. Slight variations in the control parameter can lead to either sudden or gradual changes in the system, typically referred to as first-order (abrupt or discontinuous) or second-order (smooth or continuous) phase transitions, respectively. Here, we emphasize how the phase transitions in networks characterize the critical phenomena of a complex system. Recently, percolation phase transitions<sup>43–47</sup> and Bose-Einstein condensation transitions<sup>48,49</sup> from statistical physics have gained popularity in networks. Bianconi and Barabasi<sup>48</sup> use a fitness model in a complex network and draw its analogy to the condensation transition. The percolation phase transitions in climate networks have been used to identify the signatures of El Nino precursors<sup>50</sup>, tropical cyclones<sup>51</sup>, and the weakening and expansion of the Hadley cell<sup>52</sup>.

Consider a network with  $N$  nodes that are entirely disconnected initially. The evolution of a random network (Erdos-Renyi network)<sup>53</sup> begins when a random link is added between any two given nodes. Initially, this results in only a few pairs of nodes, which then grow into trees. After a certain point, adding any more links to the network results in the connection of these isolated trees, eventually forming a giant component. The emergence of a giant component during the evolution of a random network as the average degree ( $\langle k \rangle$ ) exceeds 1 resembles a phase transition. Many properties of the network at the critical point when  $\langle k \rangle = 1$  are similar to the properties of a physical system undergoing phase transition and follow scaling behaviour<sup>54</sup>. The transition of the network from multiple isolated components to a single giant component

is analogous to the water-ice transition and magnetic phase transitions. We next discuss the different processes that explain how discontinuous phase transitions occur in networks. We then give a physical explanation to describe the phase transitions obtained in our network.

Achlioptas process<sup>55</sup> is a modified version of forming an Erdos-Renyi graph where, instead of choosing one edge at a time, two candidate edges are selected, and the consequence of each edge added separately to the graph is examined. The edge that satisfies a non-random selection rule is added to the graph, while the second candidate edge is rejected. This selection rule can either delay or accelerate the percolation transition. The generalization of this process by considering candidate edges  $m \geq 2$  at a time, where  $m$  is kept constant, is known as the Achlioptas process. The underlying mechanism to describe different types of phase transitions in networks is that the components merge using a nonrandom selection rule, which can be classified as bounded and unbounded size rules.

In a bounded-size rule, all components of size  $\geq K$ , where  $K$  is constant, are treated equivalently. One such process that involves the use of the bounded-size rule is the Bohman and Frieze (BF) process<sup>55</sup>. In the Bohman and Frieze process, the candidate edge that joins two isolated nodes is accepted, while the other candidate edge is discarded. In other words, the components with size greater than or equal to two ( $K \geq 2$ ) are treated equally as only the isolated nodes (i.e., nodes with size one) are distinguished. Based on numerical studies and mathematical considerations, Spencer and Wormald<sup>56</sup> show that for all the bounded-size rules, the percolation transition is observed to be continuous.

However, when it comes to unbounded size rules, numerical studies have shown that these rules can give rise to discontinuous percolation transitions<sup>57</sup>. One such rule is the product rule (PR)<sup>57</sup>, where two random edges are chosen, and the edge that minimises the product of the sizes of the two components is retained while the other edge is discarded. As a result, initially, there will be relatively many smaller components, and after a critical point, these components merge, and the size of the largest component increases abruptly. A similar set of results holds when the product operation is replaced by the sum in the PR rule discussed above. Therefore, enforcing a restriction on the way a component grows can alter the nature of the phase transition in networks. This percolation phase transition can further be accelerated by selecting the edge that maximizes the product of the sizes of the components in the PR rule.

In our case, we observe the second-largest component growing over Southwest India (SWI) (Main text Fig. 1a-f). Still, it merges with the giant component from the East only after the large-scale onset, which occurs over the Indian peninsula on 9<sup>th</sup> June. What could be the physical mechanism behind the restriction on the growth of the components in this case? Such restrictions can arise due to the synoptic scale activities happening in SWI prior to the large-scale onset of the monsoon. This synoptic-scale activity can be due to the weak northward propagating Monsoon Intraseasonal Oscillation (MISO), which cannot propagate northwards until the large-scale onset has occurred. Flatau et al.<sup>58</sup> and Zhou et al.<sup>59</sup> have shown that the MISOs can lead to the early onset of monsoon as well as bogus onsets depending on the active or break phase of the Intraseasonal Oscillation (ISO). The wet phase of the ISO triggers and accelerates the Monsoon onset over Kerala (MoK), while the dry phase delays the onset and induces a heat wave over India prior to the beginning of the rainy season<sup>60</sup>. However, despite these restrictions, the large-scale organization sets up after the large-scale onset, with a large fraction of an area in the southwest peninsula undergoing an abrupt onset.

In the case of large-scale onset over Northeast India (NEI), the same restriction due to synoptic-scale systems can be due to the conducive climate in May<sup>61</sup>, which is characterized by: (i) a three to four times increase in the low-level cyclonic vorticity. This increase in the magnitude of vorticity occurs due to the extratropical transient Rossby waves in May. (ii) a five to six-fold increase in the northward moisture transport from the Bay of Bengal, which sustains the monsoon heat source post-onset.

In summary, the synoptic-scale activity over NEI and the Indian peninsula restricts the merging of clusters of local onsets and, therefore, prevents the occurrence of abrupt transitions. These abrupt transitions occur only after a planetary-scale monsoon system has been established over NEI and the Indian peninsula.

## References

1. Bombardi, R. J., Moron, V. & Goodnight, J. S. Detection, variability, and predictability of monsoon onset and withdrawal dates: A review. *Int. J. Climatol* **40**, 641–667 (2020).
2. Misra, V., Bhardwaj, A. & Mishra, A. Local onset and demise of the Indian summer monsoon. *Clim. Dyn.* **51**, 1609–1622 (2018).

3. Xavier, P. K., Marzin, C. & Goswami, B. N. An objective definition of the Indian summer monsoon season and a new perspective on the ENSO–monsoon relationship. *Q. J. R. Meteorol. Soc* **133**, 749–764 (2007).
4. Saha, P., Mahanta, R. & Goswami, B. Present and future of the South Asian summer monsoon’s rainy season over Northeast India. *npj Clim. Atmos. Sci.* **6**, 170 (2023).
5. Pai, D. *et al.* Normal dates of onset/progress and withdrawal of southwest monsoon over India. *Mausam* **71**, 553–570 (2020).
6. Ananthakrishnan, R. & Soman, M. The onset of the southwest monsoon over Kerala: 1901–1980. *Int. J. Climatol* **8**, 283–296 (1988).
7. Ananthakrishnan, R. & Soman, M. The onset of the southwest monsoon in 1990. *Curr. Sci.* **61**, 447–453 (1991).
8. Pai, D. & Nair, R. M. Summer monsoon onset over Kerala: New definition and prediction. *J. Earth Syst. Sci.* **118**, 123–135 (2009).
9. Fasullo, J. & Webster, P. A Hydrological Definition of Indian Monsoon Onset and Withdrawal. *J. Clim.* **16**, 3200–3211 (2003).
10. Walker, J. M. & Bordoni, S. Onset and withdrawal of the large-scale South Asian monsoon: A dynamical definition using change point detection. *Geophys. Res. Lett.* **43**, 11–815 (2016).
11. Wang, B. *et al.* Rainy season of the Asian–Pacific summer monsoon. *J. Clim.* **15**, 386–398 (2002).
12. Von Bertalanffy, L. *General System Theory: Foundations, Development, Applications* (G. Braziller, 1968).
13. Estrada, E. What is a complex system, after all? *Foundations of Science* **29**, 1143–1170 (2024).
14. Siegenfeld, A. F. & Bar-Yam, Y. An Introduction to Complex Systems Science and Its Applications. *Complexity* **2020**, 6105872 (2020).
15. Ladyman, J., Lambert, J. & Wiesner, K. What is a complex system? *European Journal for Philosophy of Science* **3**, 33–67 (2013).

16. Franzke, C. L. & O’Kane, T. J. *Nonlinear and Stochastic Climate Dynamics* (Cambridge University Press, 2017).
17. Dijkstra, H. A., Hernández-García, E., Masoller, C. & Barreiro, M. *Networks in Climate* (Cambridge University Press, Cambridge, 2019).
18. Donner, R. V., Lindner, M., Tupikina, L. & Molkenhuth, N. Characterizing Flows by Complex Network Methods. *A Mathematical Modeling Approach from Nonlinear Dynamics to Complex Systems*, 197–226 (2019).
19. Donges, J. F., Petrova, I., Loew, A., Marwan, N. & Kurths, J. How complex climate networks complement eigen techniques for the statistical analysis of climatological data. *Clim. Dyn.* **45**, 2407–2424 (2015).
20. Fan, J. *et al.* Statistical physics approaches to the complex Earth system. *Physics reports* **896**, 1–84 (2021).
21. Ludescher, J. *et al.* Network-based forecasting of climate phenomena. *Proceedings of the National Academy of Sciences* **118**, e1922872118 (2021).
22. Sujith, R. I. & Pawar, S. A. *Thermoacoustic Instability: A Complex Systems Perspective* ISBN: 978-3-030-81134-1 (Springer, Jan. 2021).
23. Page, S. E. What Sociologists Should Know About Complexity. *Annual Review of Sociology* **41**, 21–41 (2015).
24. Arthur, W. B. Foundations of complexity economics. *Nature Reviews Physics* **3**, 136–145 (2021).
25. Tsonis, A. A., Swanson, K. L. & Wang, G. On the Role of Atmospheric Teleconnections in Climate. *J. Clim.* **21**, 2990–3001 (2008).
26. Donges, J. F., Zou, Y., Marwan, N. & Kurths, J. Complex networks in climate dynamics: Comparing linear and nonlinear network construction methods. *The European Physical Journal Special Topics* **174**, 157–179 (2009).
27. Tsonis, A. A. & Roebber, P. J. The architecture of the climate network. *Physica A: Statistical Mechanics and its Applications* **333**, 497–504 (2004).

28. Ludescher, J. *et al.* Improved El Niño forecasting by cooperativity detection. *Proceedings of the National Academy of Sciences* **110**, 11742–11745 (2013).
29. Ludescher, J. *et al.* Very early warning of next El Niño. *Proceedings of the National Academy of Sciences* **111**, 2064–2066 (2014).
30. Rodríguez-Méndez, V., Eguíluz, V. M., Hernández-García, E. & Ramasco, J. J. Percolation-based precursors of transitions in extended systems. *Scientific Reports* **6**, 29552 (2016).
31. Meng, J., Fan, J., Ashkenazy, Y., Bunde, A. & Havlin, S. Forecasting the magnitude and onset of El Niño based on climate network. *New Journal of Physics* **20**, 043036 (2018).
32. Malik, N., Bookhagen, B., Marwan, N. & Kurths, J. Analysis of spatial and temporal extreme monsoonal rainfall over South Asia using complex networks. *Clim. Dyn.* **39**, 971–987 (2012).
33. Stolbova, V., Martin, P., Bookhagen, B., Marwan, N. & Kurths, J. Topology and seasonal evolution of the network of extreme precipitation over the Indian subcontinent and Sri Lanka. *Nonlinear Processes in Geophysics* **21**, 901–917 (2014).
34. Boers, N., Bookhagen, B., Marwan, N., Kurths, J. & Marengo, J. Complex networks identify spatial patterns of extreme rainfall events of the South American Monsoon System. *Geophys. Res. Lett.* **40**, 4386–4392 (2013).
35. Boers, N. *et al.* Prediction of extreme floods in the eastern Central Andes based on a complex networks approach. *Nature communications* **5**, 5199 (2014).
36. Ciemer, C. *et al.* An early-warning indicator for Amazon droughts exclusively based on tropical Atlantic sea surface temperatures. *Environmental Research Letters* **15**, 094087 (2020).
37. Mondal, S. & Mishra, A. K. Complex networks reveal heatwave patterns and propagations over the USA. *Geophys. Res. Lett.* **48**, e2020GL090411 (2021).
38. Kretschmer, M., Coumou, D., Donges, J. F. & Runge, J. Using causal effect networks to analyze different Arctic drivers of midlatitude winter circulation. *J. Clim.* **29**, 4069–4081 (2016).
39. Malik, N., Marwan, N. & Kurths, J. Spatial structures and directionalities in Monsoonal precipitation over South Asia. *Nonlinear Processes in Geophysics* **17**, 371–381 (2010).

40. Scarsoglio, S., Laio, F. & Ridolfi, L. Climate dynamics: a network-based approach for the analysis of global precipitation. *PLoS One* **8**, e71129 (2013).
41. Boers, N. *et al.* Complex networks reveal global pattern of extreme-rainfall teleconnections. *Nature* **566**, 373–377 (2019).
42. Lübeck, S. Universal scaling behavior of non-equilibrium phase transitions. *International Journal of Modern Physics B* **18**, 3977–4118 (2004).
43. Fornito, A., Zalesky, A. & Bullmore, E. *Fundamentals of Brain Network Analysis* (Academic press, 2016).
44. Gallos, L. K., Sigman, M. & Makse, H. A. The conundrum of functional brain networks: small-world efficiency or fractal modularity. *Frontiers in Physiology* **3**, 123 (2012).
45. Deb, D., Vishveshwara, S. & Vishveshwara, S. Understanding Protein Structure from a Percolation Perspective. *Biophysical Journal* **97**, 1787–1794 (2009).
46. Weber, J. K. & Pande, V. S. Percolation-like phase transitions in network models of protein dynamics. *The Journal of Chemical Physics* **142** (2015).
47. Lu, Z., Yuan, N. & Fu, Z. Percolation Phase Transition of Surface Air Temperature Networks under Attacks of El Niño/La Niña. *Scientific Reports* **6**, 26779 (2016).
48. Bianconi, G. & Barabási, A.-L. Bose-Einstein Condensation in Complex Networks. *Physical review letters* **86**, 5632 (2001).
49. Tang, M., Liu, L. & Liu, Z. Influence of dynamical condensation on epidemic spreading in scale-free networks. *Physical Review E—Statistical, Nonlinear, and Soft Matter Physics* **79**, 016108 (2009).
50. Sonone, R. & Gupte, N. Precursors of the El Niño phenomenon: A climate network analysis. *Physical Review E* **103**, L040301 (2021).
51. Sonone, R. & Gupte, N. Climate network analysis of extreme events: Tropical cyclones. *Chaos: An Interdisciplinary Journal of Nonlinear Science* **34** (2024).
52. Fan, J., Meng, J., Ashkenazy, Y., Havlin, S. & Schellnhuber, H. J. Climate network percolation reveals the expansion and weakening of the tropical component under global warming. *Proceedings of the National Academy of Sciences* **115**, E12128–E12134 (2018).

53. Erdos, P. & Renyi, A. On random graphs I. *Publ. math. debrecen* **6**, 18 (1959).
54. Barabási, A. & Pósfai, M. *Network Science* (Cambridge University Press, Cambridge, 2016).
55. Bohman, T. & Frieze, A. Avoiding a giant component. *Random Structures & Algorithms* **19**, 75–85 (2001).
56. Spencer, J. & Wormald, N. Birth control for giants. *Combinatorica* **27**, 587–628 (2007).
57. Achlioptas, D., D’Souza, R. M. & Spencer, J. Explosive Percolation in Random Networks. *Science* **323**, 1453–1455 (2009).
58. Flatau, M. K., Flatau, P. J. & Rudnick, D. The Dynamics of Double Monsoon Onsets. *J. Clim.* **14**, 4130–4146 (2001).
59. Zhou, L. & Murtugudde, R. Impact of northward-propagating intraseasonal variability on the onset of Indian summer monsoon. *J. Clim.* **27**, 126–139 (2014).
60. Wang, B., Ding, Q. & Joseph, P. Objective Definition of the Indian Summer Monsoon Onset. *J. Clim.* **22**, 3303–3316 (2009).
61. Das, S., Goswami, D. J., Mahanta, R., Saha, P. & Goswami, B. Dynamics of May ‘onset’ of Indian summer monsoon over Northeast India. *Quarterly Journal of the Royal Meteorological Society* **150**, 4533–4549 (2024).
